# Supplementary material for: Classification of critical phenomena in hierarchical small-world networks
Source: arXiv:1209.3447 source file (2015-05-08)
Supplement: Supplementary file 1 [file HN5y_supplement.pdf]

# Supplement B:

## “Classification of Critical Phenomena having a Parameter-Dependent Renormalization ”

S. Boettcher and C. T. Brunson

---

### Ising Hamiltonian for Hanoi Network HN5:

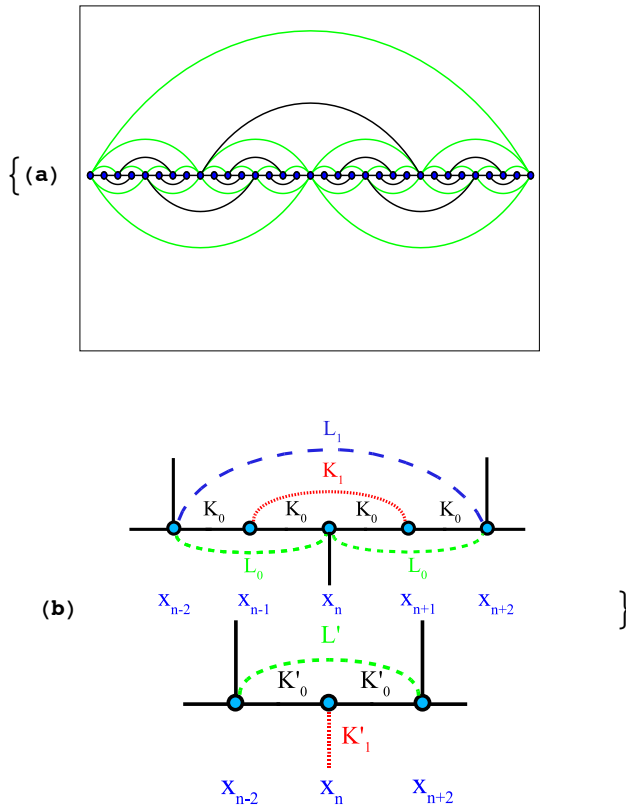

Figure (a) displays the network HN5 (here, with N=33 nodes). The Ising Hamiltonian on this network is

$$\begin{aligned}
 -\beta \mathcal{H} = & K_0(x_0 x_1 + x_1 x_2 + \dots + x_{N-1} x_N) + \\
 & K_1[(x_1 x_3 + x_5 x_7 + \dots + x_{N-3} x_{N-1}) + (x_2 x_6 + x_{10} x_{14} + \dots + x_{N-6} x_{N-2}) + \dots + (x_{N/4} x_{3N/4})] + \\
 & L[(x_0 x_2 + x_2 x_4 + \dots + x_{N-2} x_N) + (x_0 x_4 + x_4 x_8 + \dots + x_{N-4} x_N) + \dots + (x_0 x_{N/2} + x_{N/2} x_N) + (x_0 x_N)] + H(x_0 + \dots + x_N)
 \end{aligned}$$

with raw couplings  $K_0 = K_1 = \beta J$ ,  $L = L_0 = L_1 = y\beta J$ , and field  $H = \beta h$ . The parameter  $y \in [0, 1]$  allows to define the strength of long-range couplings (marked green in the equation and figure (a)) relative to those in the 1d-backbone of the network,  $L = yK_0$ .

A single renormalization group (RG) step consists of tracing out every 2nd spin, and we regroup the Hamiltonian into those terms containing all odd-index spins and the rest:

$$-\beta\mathcal{H} = \sum_n (-\beta\mathcal{H}_n) + R(\mathbf{x}_0, \mathbf{x}_2, \dots, \mathbf{x}_{N-2}, \mathbf{x}_N)$$

with the “sectional” Hamiltonians  $-\beta\mathcal{H}_n$  for  $n=2(2j-1)$ , running over all sections  $j=1,2,\dots,N/4$ . The top of figure (b) shows the spins and their couplings in each such section of the network. The RG-step consists of tracing out the odd-index spins,  $\mathbf{x}_{n-1}$  and  $\mathbf{x}_{n+1}$ , in each section. We define “activities”  $\mu=\exp\{-2\beta J\}$  and  $\eta=\exp\{-\beta h\}$  and parametrize the renormalizable couplings in terms “raw” activities  $A_0 = 0$ ,  $A_1 = \mu^2$ ,  $A_2 = \mu^2 \eta$ ,  $A_3 = \eta$ ,  $A_4 = 1$ , and  $A_5 = 1$ , where  $A_0$  becomes the renormalized energy scale,  $A_1 = \exp\{-2K_0\}$  and  $A_2 = \exp\{-2L\}$  are the renormalized backbone and long-range couplings,  $A_3 = \exp\{-H_s\}$  and  $A_4 = \exp\{-H_b\}$  are the renormalized site- and bond-magnetizations (initially,  $H_s = H$  and  $H_b = 0$ ), and  $A_5$  is the renormalized 3-point magnetization which arises in this RG when the up/down symmetry is broken by the external field. With  $A_1$  representing the coupling strength along the backbone of HN5, its behavior resembles most closely that of  $\kappa$  in our theory.

Then, we can write the sectional Hamiltonian as  $Z_0 = \exp\{-\beta\mathcal{H}_n\}$  before the RG-step at any point during the RG recursion as

```
In[1]:= Z0[x0_, x1_, x2_, x3_, x4_] := Exp[-A0] *
  A1 ^ (- (x0 * x1 + x1 * x2 + x2 * x3 + x3 * x4) / 4) * mu ^ (- (x1 * x3) / 2) *
  A2 ^ (- (x0 * x2 + x2 * x4) / 4) * mu ^ (- y (x0 * x4) / 2) *
  A3 ^ (- ((x0 + x1) + (x1 + x2) + (x2 + x3) + (x3 + x4)) / 4) *
  A4 ^ (- ((x0 + x2) + (x2 + x4)) / 4) *
  A5 ^ (- (x0 * x1 * x2 + x2 * x3 * x4) / 2)
```

Notice the explicit dependence on the raw activity  $\mu$  originating with the long-range couplings  $K_1$  that do not get renormalized, see Figure (b) above.

---

## Obtaining the RG-flow:

The RG-step consists of tracing out the odd-index spins in  $Z_0$  from before the RG-step, and express the result in a function  $Z_1$  after the RG-step that is identical in shape (see bottom of figure (b)), i.e.,

```
In[2]:= Z1[x0_, x2_, x4_] := Exp[-B0 / 2] *
  B1 ^ (- (x0 * x2 + x2 * x4) / 4) *
  B2 ^ (- (x0 * x4) / 4) *
  B3 ^ (- ((x0 + x2) + (x2 + x4)) / 4) *
  B4 ^ (- (x0 * x4) / 4) *
  B5 ^ (- (x0 * x2 * x4) / 2)
```

where the  $B_i$  are the newly renormalized activities. To this end, we require  $Z_1[\mathbf{x}_{n-2}, \mathbf{x}_n, \mathbf{x}_{n+2}] = \sum_{\mathbf{x}_{n-1}} \sum_{\mathbf{x}_{n+1}} Z_0[\mathbf{x}_{n-2}, \mathbf{x}_{n-1}, \mathbf{x}_n, \mathbf{x}_{n+1}, \mathbf{x}_{n+2}]$ :

```
In[3]:= TrZ0[x0_, x2_, x4_] := Sum[Sum[Z0[x0, x1, x2, x3, x4], {x1, -1, 1, 2}], {x3, -1, 1, 2}]
```

Hence, both sides have to be equal for all combinations of  $\mathbf{x}_{n-2}, \mathbf{x}_n, \mathbf{x}_{n+2} = + / - 1$ ,

```

In[4]:= i = 0;
For[xn-2 = -1, xn-2 ≤ 1, xn-2 += 2, For[xn = -1, xn ≤ 1, xn += 2, For[xn+2 = -1, xn+2 ≤ 1, xn+2 += 2,
  leq[i] = Z1[xn-2, xn, xn+2];
  req[i++] = Factor[TrZ0[xn-2, xn, xn+2]];
]]]
leq[0] == req[0]
leq[1] == req[1]
leq[2] == req[2]
leq[3] == req[3]
leq[4] == req[4]
leq[5] == req[5]
leq[6] == req[6]
leq[7] == req[7]

```

$$\text{Out[6]} = \frac{e^{-\frac{B_0}{2}} B_3 \sqrt{B_4} \sqrt{B_5}}{\sqrt{B_1} B_2^{1/4}} = \frac{e^{-A_0} \mu^{-\frac{1}{2} - \frac{y}{2}} A_4 (A_1^2 + 2 \mu A_1 A_3 A_5 + A_3^2 A_5^2)}{A_1 \sqrt{A_2} A_5}$$

$$\text{Out[7]} = \frac{e^{-\frac{B_0}{2}} B_2^{1/4} \sqrt{B_3}}{\sqrt{B_5}} = \frac{e^{-A_0} \mu^{-\frac{1}{2} - \frac{y}{2}} \sqrt{A_4} (\mu A_1 A_3 + A_1 A_5 + A_3^2 A_5 + \mu A_3 A_5^2)}{\sqrt{A_1} \sqrt{A_3} A_5}$$

$$\text{Out[8]} = \frac{e^{-\frac{B_0}{2}} \sqrt{B_1} \sqrt{B_4}}{B_2^{1/4} \sqrt{B_5}} = \frac{e^{-A_0} \mu^{-\frac{1}{2} - \frac{y}{2}} \sqrt{A_2} (A_3^2 + 2 \mu A_3 A_5 + A_5^2)}{A_3 A_5}$$

$$\text{Out[9]} = \frac{e^{-\frac{B_0}{2}} B_2^{1/4} \sqrt{B_5}}{\sqrt{B_3}} = \frac{e^{-A_0} \mu^{-\frac{1}{2} - \frac{y}{2}} (\mu A_3 + A_5 + A_1 A_3^2 A_5 + \mu A_1 A_3 A_5^2)}{\sqrt{A_1} A_3^{3/2} \sqrt{A_4} A_5}$$

$$\text{Out[10]} = \frac{e^{-\frac{B_0}{2}} B_2^{1/4} \sqrt{B_3}}{\sqrt{B_5}} = \frac{e^{-A_0} \mu^{-\frac{1}{2} - \frac{y}{2}} \sqrt{A_4} (\mu A_1 A_3 + A_1 A_5 + A_3^2 A_5 + \mu A_3 A_5^2)}{\sqrt{A_1} \sqrt{A_3} A_5}$$

$$\text{Out[11]} = \frac{e^{-\frac{B_0}{2}} \sqrt{B_1} \sqrt{B_5}}{B_2^{1/4} \sqrt{B_4}} = \frac{e^{-A_0} \mu^{-\frac{1}{2} - \frac{y}{2}} \sqrt{A_2} (A_3^2 + 2 \mu A_3 A_5 + A_5^2)}{A_3 A_5}$$

$$\text{Out[12]} = \frac{e^{-\frac{B_0}{2}} B_2^{1/4} \sqrt{B_5}}{\sqrt{B_3}} = \frac{e^{-A_0} \mu^{-\frac{1}{2} - \frac{y}{2}} (\mu A_3 + A_5 + A_1 A_3^2 A_5 + \mu A_1 A_3 A_5^2)}{\sqrt{A_1} A_3^{3/2} \sqrt{A_4} A_5}$$

$$\text{Out[13]} = \frac{e^{-\frac{B_0}{2}}}{\sqrt{B_1} B_2^{1/4} B_3 \sqrt{B_4} \sqrt{B_5}} = \frac{e^{-A_0} \mu^{-\frac{1}{2} - \frac{y}{2}} (1 + 2 \mu A_1 A_3 A_5 + A_1^2 A_3^2 A_5^2)}{A_1 \sqrt{A_2} A_3^2 A_4 A_5}$$

Due to the remaining symmetries, not all of these relations are independent. In fact, since there are 6 renormalizable couplings, there are also six independent relations. (To simplify the task for *Mathematica*, it is advisable to eliminate unnecessary dependences before solving!)

```

In[14]:= SB[0] = Expand[Solve[Log[leq[0] * leq[1] * leq[2] * leq[3] * leq[4] * leq[5] * leq[6] * leq[7]] ==
  Log[Simplify[req[0] * req[1] * req[2] * req[3] * req[4] *
    req[5] * req[6] * req[7] * Exp[8 * A0]]] - 8 * A0, B0]][[1]]
SB[1] = PowerExpand[Simplify[Solve[Factor[(leq[2] * leq[5]) / (leq[0] * leq[7])] ==
  Factor[(req[2] * req[5]) / (req[0] * req[7])], B1]][[2]]]
SB[2] = PowerExpand[Simplify[Solve[Factor[(leq[1]^2 * leq[3]^2) /
  (leq[2] * leq[5] * leq[0] * leq[7])] ==
  Factor[(req[1]^2 * req[3]^2) / (req[2] * req[5] * req[0] * req[7])], B2]][[2]]]
SB[3] = PowerExpand[Simplify[Solve[Factor[(leq[1]^2 * leq[0] * leq[5]) /
  (leq[3]^2 * leq[7] * leq[2])] ==
  Factor[(req[1]^2 * req[0] * req[5]) / (req[3]^2 * req[7] * req[2])], B3]][[4]]]
SB[4] = PowerExpand[Simplify[Solve[Factor[(leq[3]^2 * leq[2]^3 * leq[0]) /
  (leq[5]^3 * leq[1]^2 * leq[7])] ==
  Factor[(req[3]^2 * req[2]^3 * req[0]) / (req[5]^3 * req[1]^2 * req[7])], B4]][[4]]]
SB[5] = PowerExpand[Simplify[Solve[Factor[(leq[3]^2 * leq[0] * leq[5]) /
  (leq[1]^2 * leq[7] * leq[2])] ==
  Factor[(req[3]^2 * req[0] * req[5]) / (req[1]^2 * req[7] * req[2])], B5]][[4]]]

RGh=0 = Table[Part[SB[n], 1], {n, 0, 5}];

```

$$\begin{aligned}
\text{Out[14]} = & \left\{ B_0 \rightarrow \text{Log}[\mu] + \text{Log}[A_1] + 2 \text{Log}[A_3] + 2 \text{Log}[A_5] - \frac{1}{2} \text{Log}[A_3^2 + 2 \mu A_3 A_5 + A_5^2] - \right. \\
& \frac{1}{4} \text{Log}[A_1^2 + 2 \mu A_1 A_3 A_5 + A_3^2 A_5^2] - \frac{1}{4} \text{Log}[1 + 2 \mu A_1 A_3 A_5 + A_1^2 A_3^2 A_5^2] - \\
& \left. \frac{1}{2} \text{Log}[A_1 (\mu A_3 + A_5) + A_3 A_5 (A_3 + \mu A_5)] - \frac{1}{2} \text{Log}[A_5 + A_1 A_3^2 A_5 + A_3 (\mu + \mu A_1 A_5^2)] + 2 A_0 \right\}
\end{aligned}$$

$$\begin{aligned}
\text{Out[15]} = & \left\{ B_1 \rightarrow \left( A_1 A_2 (A_3^2 + 2 \mu A_3 A_5 + A_5^2) \right) / \right. \\
& \left( \sqrt{A_3^2 A_5^2 + A_1^4 A_3^2 A_5^2 + 2 \mu A_1 A_3 A_5 (1 + A_3^2 A_5^2)} + 2 \mu A_1^3 A_3 A_5 (1 + A_3^2 A_5^2) + A_1^2 (1 + 4 \mu^2 A_3^2 A_5^2 + A_3^4 A_5^4) \right) \left. \right\}
\end{aligned}$$

$$\begin{aligned}
\text{Out[16]} = & \left\{ B_2 \rightarrow \left( \mu^{2y} (A_1 (\mu A_3 + A_5) + A_3 A_5 (A_3 + \mu A_5)) (A_5 + A_1 A_3^2 A_5 + A_3 (\mu + \mu A_1 A_5^2)) \right) / \right. \\
& \left( (A_3^2 + 2 \mu A_3 A_5 + A_5^2) \sqrt{A_1^2 + 2 \mu A_1 A_3 A_5 + A_3^2 A_5^2} \sqrt{1 + 2 \mu A_1 A_3 A_5 + A_1^2 A_3^2 A_5^2} \right) \left. \right\}
\end{aligned}$$

$$\begin{aligned}
\text{Out[17]} = & \left\{ B_3 \rightarrow \left( A_3 A_4 (A_1^2 + 2 \mu A_1 A_3 A_5 + A_3^2 A_5^2)^{1/4} \sqrt{A_1 (\mu A_3 + A_5) + A_3 A_5 (A_3 + \mu A_5)} \right) / \right. \\
& \left( (1 + 2 \mu A_1 A_3 A_5 + A_1^2 A_3^2 A_5^2)^{1/4} \sqrt{A_5 + A_1 A_3^2 A_5 + A_3 (\mu + \mu A_1 A_5^2)} \right) \left. \right\}
\end{aligned}$$

$$\begin{aligned}
\text{Out[18]} = & \left\{ B_4 \rightarrow \left( (A_1^2 + 2 \mu A_1 A_3 A_5 + A_3^2 A_5^2)^{1/4} \sqrt{A_5 + A_1 A_3^2 A_5 + A_3 (\mu + \mu A_1 A_5^2)} \right) / \right. \\
& \left( (1 + 2 \mu A_1 A_3 A_5 + A_1^2 A_3^2 A_5^2)^{1/4} \sqrt{A_1 (\mu A_3 + A_5) + A_3 A_5 (A_3 + \mu A_5)} \right) \left. \right\}
\end{aligned}$$

$$\begin{aligned}
\text{Out[19]} = & \left\{ B_5 \rightarrow \left( (A_1^2 + 2 \mu A_1 A_3 A_5 + A_3^2 A_5^2)^{1/4} \sqrt{A_5 + A_1 A_3^2 A_5 + A_3 (\mu + \mu A_1 A_5^2)} \right) / \right. \\
& \left( (1 + 2 \mu A_1 A_3 A_5 + A_1^2 A_3^2 A_5^2)^{1/4} \sqrt{A_1 (\mu A_3 + A_5) + A_3 A_5 (A_3 + \mu A_5)} \right) \left. \right\}
\end{aligned}$$

These are the RG-flow equations. Again, notice the dependence on the temperature  $\beta$  through the explicit occurrence of  $\mu$ .

As mentioned above, the RG-flow is initiated through the raw couplings via

```

In[21]:= SIC = {B0 -> 0, B1 -> mu^2, B2 -> mu^2 y, B3 -> eta, B4 -> 1, B5 -> 1}

```

```

Out[21]= {B0 -> 0, B1 -> mu^2, B2 -> mu^2 y, B3 -> eta, B4 -> 1, B5 -> 1}

```

---

## Fixed Points at h=0:

First, we consider the case  $h=0$  ( $\eta=1$ ), in which case the RG-flow for the activities  $A_3$ ,  $A_4$ , and  $A_5$  become trivial:

In[22]:= **RG<sub>h0</sub> = FullSimplify[RG<sub>h→0</sub> /. η → 1 /. A<sub>3</sub> → 1 /. A<sub>4</sub> → 1 /. A<sub>5</sub> → 1, Assumptions → μ > 0 && y > 0 && A<sub>1</sub> > 0 && A<sub>2</sub> > 0]**

$$\text{Out[22]} = \left\{ B_0 \rightarrow \text{Log}[\mu] + \text{Log}[A_1] + \frac{1}{2} \text{Log}\left[\frac{1}{2(1+\mu)^3(1+A_1)^2(1+2\mu A_1+A_1^2)}\right] + 2A_0, \right. \\ \left. B_1 \rightarrow \frac{2(1+\mu)A_1A_2}{1+2\mu A_1+A_1^2}, B_2 \rightarrow \frac{\mu^{2y}(1+\mu)(1+A_1)^2}{2(1+2\mu A_1+A_1^2)}, B_3 \rightarrow 1, B_4 \rightarrow 1, B_5 \rightarrow 1 \right\}$$

The recursions for  $A_1$  and  $A_2$  correspond to those for  $\kappa$  and  $\lambda$  in Eq. (19) of Ref. [Boettcher&Brunson, 2011]. We obtain the fixed points by equating  $B_i = A_i$  in the RG-flow:

In[23]:= **FP = FullSimplify[Solve[({B<sub>1</sub>, B<sub>2</sub>} /. RG<sub>h0</sub>) == {A<sub>1</sub>, A<sub>2</sub>}, {A<sub>1</sub>, A<sub>2</sub>}], Assumptions → μ > 0 && y > 0]**

$$\text{Out[23]} = \left\{ \left\{ A_1 \rightarrow 0, A_2 \rightarrow \frac{1}{2} \mu^{2y} (1+\mu) \right\}, \left\{ A_1 \rightarrow \frac{1}{2} \left( \mu^y + \mu(-2+\mu^y) - \sqrt{-4+4\mu^2+\mu^{2y}(1+\mu)^2-4\mu^y(-1+\mu^2)} \right), \right. \right. \\ \left. A_2 \rightarrow \frac{1}{4} \mu^y \left( 2+\mu^y+\mu(-2+\mu^y) - \sqrt{-4+4\mu^2+\mu^{2y}(1+\mu)^2-4\mu^y(-1+\mu^2)} \right) \right\}, \\ \left\{ A_1 \rightarrow \frac{1}{2} \left( \mu^y + \mu(-2+\mu^y) + \sqrt{-4+4\mu^2+\mu^{2y}(1+\mu)^2-4\mu^y(-1+\mu^2)} \right), \right. \\ \left. A_2 \rightarrow \frac{1}{4} \mu^y \left( 2+\mu^y+\mu(-2+\mu^y) + \sqrt{-4+4\mu^2+\mu^{2y}(1+\mu)^2-4\mu^y(-1+\mu^2)} \right) \right\}, \\ \left\{ A_1 \rightarrow \frac{1}{2} \left( -2\mu - \mu^y(1+\mu) - \sqrt{-4+4\mu^2+\mu^{2y}(1+\mu)^2+4\mu^y(-1+\mu^2)} \right), \right. \\ \left. A_2 \rightarrow \frac{1}{4} \mu^y \left( -2+\mu^y+\mu(2+\mu^y) + \sqrt{-4+4\mu^2+\mu^{2y}(1+\mu)^2+4\mu^y(-1+\mu^2)} \right) \right\}, \\ \left\{ A_1 \rightarrow \frac{1}{2} \left( -2\mu - \mu^y(1+\mu) + \sqrt{-4+4\mu^2+\mu^{2y}(1+\mu)^2+4\mu^y(-1+\mu^2)} \right), \right. \\ \left. A_2 \rightarrow \frac{1}{4} \mu^y \left( -2+\mu^y+\mu(2+\mu^y) - \sqrt{-4+4\mu^2+\mu^{2y}(1+\mu)^2+4\mu^y(-1+\mu^2)} \right) \right\} \right\}$$

A plot of the FP for the backbone activity  $A_1$  ( $= \kappa$ ) as a function of  $\mu$  for various values of  $y$  exhibits exactly the same behavior as our model, see Fig. 1(b-d) for comparison:

```

In[24]:= Show[
  Plot[μ, {μ, 0, 1}, PlotStyle → Green],
  Plot[-1 + √(2 - 2 μ), {μ, 0, 1}, PlotStyle → {Dashed}],
  Plot[{A1 /. (FP /. y → .1), A1 /. (FP /. y → .4), A1 /. (FP /. y → 1)}, {μ, 0, 1},
    PlotStyle → Thick, ColorFunction → Function[{a, b}, If[b < -1 + √(2 - 2 a), Red, Black]],
    ColorFunctionScaling → False]
, PlotRange → {{0, 1}, {-0.2, 1}}, AxesLabel → {"μ", "κ"}]

```

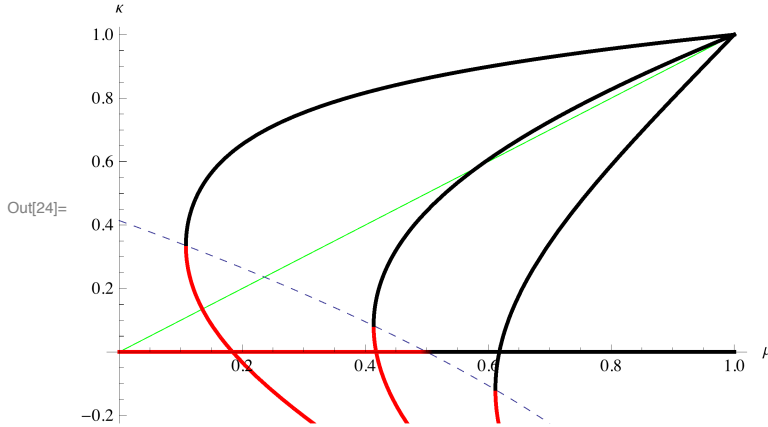

Notice that we have included in the plot (as a dashed line) the function for the location of the branch-point,

$A_1(\mu_B) = \kappa_B(\mu_B) = -1 + \sqrt{2 - 2\mu_B}$ , which results from the vanishing of the discriminant in the FP of  $A_1$ . To this end, we define a general procedure which evaluates any input quantity as a function of  $\mu_B$  ...

```

In[25]:= OnMuB[exp_] := Block[{res, Defz, Solz, z, ψ, τ},
  Defz = Collect[(-4 + 4 μy (1 + μ) + (-2 μ + μy (1 + μ))2) / μy (1 + μ) → z, z];
  Solz = Simplify[Solve[Defz == 0, z]][[2]];
  res = Factor[Simplify[exp /. y → Log[z / (1 + μ)] / Log[μ], Assumptions → z > 0 && μ > 0]];
  res = FullSimplify[res /. Solz, Assumptions → μ < 1 && μ > 0];
  res = FullSimplify[res /. μ → 1 - τ2, Assumptions → τ > 0];
  res = FullSimplify[res /. τ → ψ + Sqrt[2], Assumptions → ψ > 0];
  res = FullSimplify[res /. ψ → Sqrt[1 - μ] - Sqrt[2], Assumptions → μ > 0];
  Return[res /. μ → μB];
]

```

...and use it to determine  $\kappa_B(\mu_B)$  from the upper branch of fixed points (FP),  $A_1 = \kappa_+(\mu) \rightarrow \kappa_B(\mu_B)$  for  $\mu \rightarrow \mu_B$ :

```

In[26]:= OnMuB[A1 /. FP[[3]]]

```

```

Out[26]= -1 + √(2 - 2 μB)

```

Now we evaluate the eigenvalues  $\lambda$  as in Eq. (7) from the Jacobian defined in Eq. (3) at  $h=0$ :

```

In[27]:= MatrixForm[
  (R')h0 = Table[FullSimplify[D[(Bi /. RGh→0) /. η → 1 /. A3 → 1 /. A4 → 1 /. A5 → 1], Aj],
    Assumptions → μ > 0 && y > 0 && A1 > 0 && A2 > 0], {j, 1, 2}, {i, 1, 2}]

```

Out[27]/MatrixForm=

$$\begin{pmatrix} -\frac{2(1+\mu)(-1+A_1^2)A_2}{(1+2\mu A_1+A_1^2)^2} & \frac{\mu^{2y}(-1+\mu^2)(-1+A_1^2)}{(1+2\mu A_1+A_1^2)^2} \\ \frac{2(1+\mu)A_1}{1+2\mu A_1+A_1^2} & 0 \end{pmatrix}$$

with eigenvalues (very long outputs have been suppressed!)

```
In[28]:= EVh0 = Eigenvalues[(R')h0];
λ0 = Simplify[(EVh0 /. FP[[1]]) , Assumptions → μ > 0 && y > 0]
λ+ = Simplify[(EVh0 /. FP[[2]]) , Assumptions → μ > 0 && y > 0];
λ- = Simplify[(EVh0 /. FP[[3]]) , Assumptions → μ > 0 && y > 0];
```

```
Out[29]:= {μ2 y (1 + μ)2, 0}
```

From those relations, we can reproduce the eigenvalue-plot in Fig. 2(b) for a branch point in the physical regime,  
 $\kappa_B(\mu_B) > 0$ :

```
In[32]:= Ev = {λ0, λ+, λ-} /. y → 0.1;
Show[
  Plot[1, {μ, 0, 1}, PlotStyle → Dashed],
  Plot[Ev, {μ, 0, 1}, PlotStyle → Thick,
    ColorFunction → Function[{a, b}, If[b > 1, Red, Black]], ColorFunctionScaling → False],
  PlotRange → {{0, 1}, {-0.3, 1.15}}, AxesLabel → {"μ", "λ"}]
```

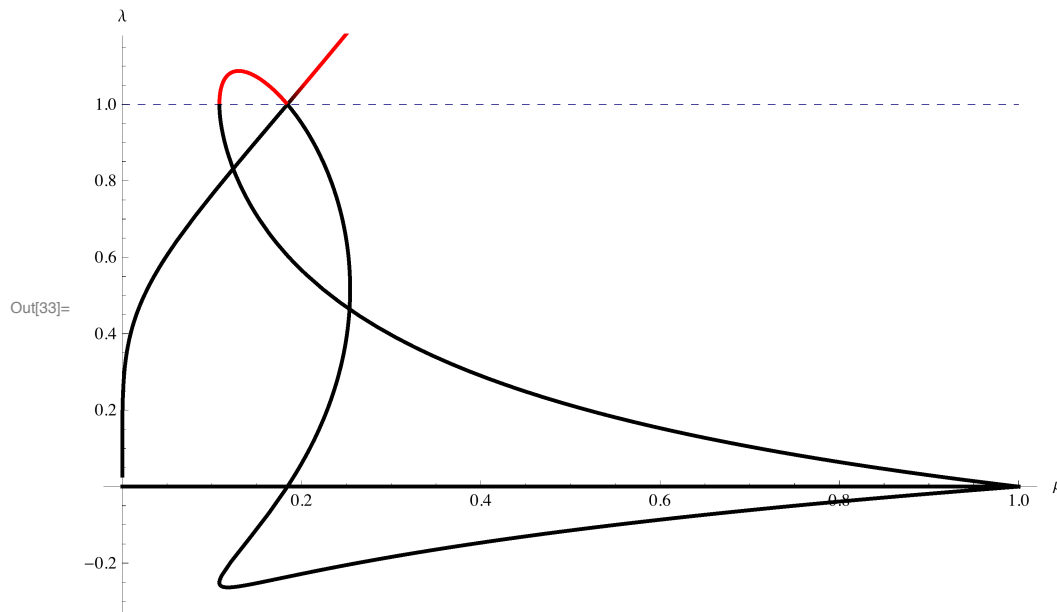

...or the corresponding plot at the critical value of  $y_c = \log_2(3/2)$  when  $\kappa_B(\mu_B) = 0$ :

```
In[34]:= Ev = {λ0, λ+, λ-} /. y → Log[3 / 2] / Log[2];
Show[
  Plot[1, {μ, 0, 1}, PlotStyle → Dashed],
  Plot[Ev, {μ, 0, 1}, PlotStyle → Thick,
    ColorFunction → Function[{a, b}, If[b > 1, Red, Black]], ColorFunctionScaling → False],
  PlotRange → {{0, 1}, {-0.2, 1.15}}, AxesLabel → {"μ", "λ"}]
```

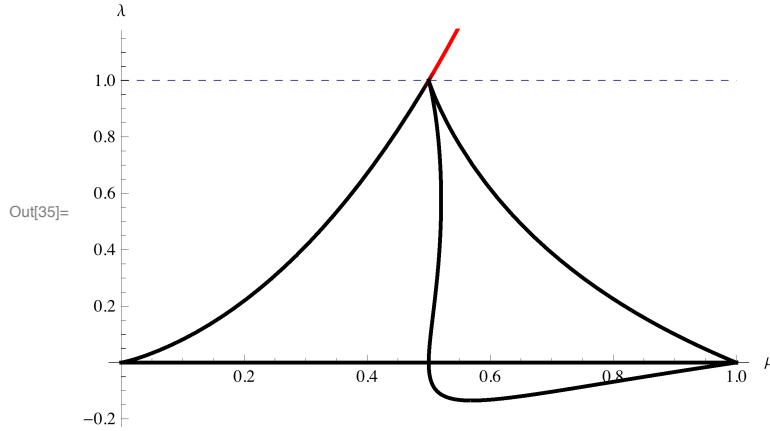

...or for  $y=1$  (somewhat enlarged) when the branch point is below the physical regime,  $\kappa_B(\mu_B) < 0$ , and  $\lambda_+$ ,  $\lambda_-$  have switched order:

```
In[36]:= Ev = {λ0, λ+, λ-} /. y → 1;
Show[
  Plot[1, {μ, 0.61, 0.63}, PlotRange → {{0.61, 0.628}, {.8, 1.05}}, PlotStyle → Dashed],
  Plot[Ev, {μ, 0.61, 0.63}, PlotRange → {{0.61, 0.628}, {.8, 1.05}}, PlotStyle → Thick,
    ColorFunction → Function[{a, b}, If[b > 1, Red, Black]], ColorFunctionScaling → False],
  AxesLabel → {"μ", "λ"}]
```

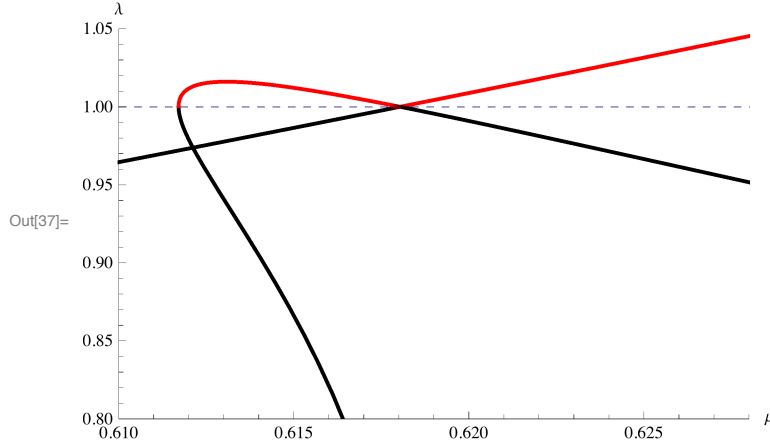

## Fixed Points at $h \rightarrow 0$ :

Inducing a magnetization for a small external field  $h \rightarrow 0$  breaks the up/down ( $Z_2$ )-symmetry and requires three new parameters, the activities  $A_3$ ,  $A_4$ , and  $A_5$  above, to be renormalized, and we arrive at the extended RG-flow,  $RG_{h \rightarrow 0}$  above. For any  $h > 0$ , the RG-flow evolves to the stable strong-field fixed point with  $A_3 = 0$ ; the behavior for small external field  $h \rightarrow 0$  is governed by the unstable fixed point  $A_3 = A_4 = A_5 = 1$  (leaving  $A_1$ ,  $A_2$  unevaluated for now), where we obtain the extended Jakobian matrix

```
In[38]:= MatrixForm[(R')_{h→0} = Table[FullSimplify[D[(B_i /. RG_{h→0}), A_j] /. A_3 → 1 /. A_4 → 1 /. A_5 → 1,
Assumptions → μ > 0 && γ > 0 && A_1 > 0 && A_2 > 0], {j, 1, 5}, {i, 1, 5}]]
```

```
Out[38]//MatrixForm=
```

$$\begin{pmatrix} -\frac{2(1+\mu)(-1+A_1^2)A_2}{(1+2\mu A_1+A_1^2)^2} & \frac{\mu^2 \gamma (-1+\mu^2)(-1+A_1^2)}{(1+2\mu A_1+A_1^2)^2} & 0 & 0 & 0 \\ \frac{2(1+\mu)A_1}{1+2\mu A_1+A_1^2} & 0 & 0 & 0 & 0 \\ 0 & 0 & \frac{1}{2} - \frac{1}{1+\mu} + \frac{2}{(1+\mu)(1+A_1)} + \frac{1+\mu A_1}{1+2\mu A_1+A_1^2} & -\frac{(-1+\mu)(-1+A_1)^3}{2(1+\mu)(1+A_1)(1+2\mu A_1+A_1^2)} & -\frac{1}{2} \\ 0 & 0 & 1 & 0 & 0 \\ 0 & 0 & -\frac{3}{2} + \frac{1}{1+\mu} + \frac{2\mu}{(1+\mu)(1+A_1)} + \frac{1+\mu A_1}{1+2\mu A_1+A_1^2} & \frac{1}{2} - \frac{1}{1+\mu} - \frac{2\mu}{(1+\mu)(1+A_1)} + \frac{1+\mu A_1}{1+2\mu A_1+A_1^2} & \frac{1}{2} - \frac{1}{1+\mu} \end{pmatrix}$$

The upper block for  $A_1, A_2$  is identical to the 2x2 matrix above, and is decoupled from the field-dependent lower block. Just focusing on the lower block:

```
In[39]:= MatrixForm[(R')_{h→0} = Table[FullSimplify[D[(B_i /. RG_{h→0}), A_j] /. A_3 → 1 /. A_4 → 1 /. A_5 → 1,
Assumptions → μ > 0 && γ > 0 && A_1 > 0 && A_2 > 0], {j, 3, 5}, {i, 3, 5}]]
```

```
Out[39]//MatrixForm=
```

$$\begin{pmatrix} \frac{1}{2} - \frac{1}{1+\mu} + \frac{2}{(1+\mu)(1+A_1)} + \frac{1+\mu A_1}{1+2\mu A_1+A_1^2} & -\frac{(-1+\mu)(-1+A_1)^3}{2(1+\mu)(1+A_1)(1+2\mu A_1+A_1^2)} & -\frac{(-1+\mu)(-1+A_1)^3}{2(1+\mu)(1+A_1)(1+2\mu A_1+A_1^2)} \\ 1 & 0 & 0 \\ -\frac{3}{2} + \frac{1}{1+\mu} + \frac{2\mu}{(1+\mu)(1+A_1)} + \frac{1+\mu A_1}{1+2\mu A_1+A_1^2} & \frac{1}{2} - \frac{1}{1+\mu} - \frac{2\mu}{(1+\mu)(1+A_1)} + \frac{1+\mu A_1}{1+2\mu A_1+A_1^2} & \frac{1}{2} - \frac{1}{1+\mu} - \frac{2\mu}{(1+\mu)(1+A_1)} + \frac{1+\mu A_1}{1+2\mu A_1+A_1^2} \end{pmatrix}$$

...provides the eigenvalues:

```
In[40]:= EV_{h→0} = FullSimplify[Eigenvalues[(R')_{h→0}], Assumptions → μ > 0 && A_1 > 0]
```

```
Out[40]= {0, \frac{(-1+\mu)(-1+A_1)}{(1+\mu)(1+A_1)}, \frac{2+2\mu A_1}{1+2\mu A_1+A_1^2}}
```

For physical  $\mu$  and fixed points of  $A_1$ , the dominant eigenvalue is

```
In[41]:= λ_h = (EV_{h→0})[[3]]
```

```
Out[41]= \frac{2+2\mu A_1}{1+2\mu A_1+A_1^2}
```

Note that  $\lambda_h \leq 2$ , and in particular,  $\lambda_h = 2$  for the fixed point with  $A_1 = \kappa_+(\mu_c) = 0$ . For  $A_1 > 0$ , it is

```
In[42]:= Series[λ_h, {A_1, 0, 1}]
```

```
Out[42]= 2 - 2\mu A_1 + O[A_1]^2
```

for any  $\gamma$ , in accordance with Eq. (12).

## Determination of magnetic exponent $\beta$ for HN5 at $\gamma=0.1$ :

We can now use the above quantities to determine, for example, the magnetic exponent of the Ising model on HN5 at  $\gamma=0.1$ , that was given as  $\beta=0.205\dots$  in Fig. 3(a). To this end, we first have to locate the critical point  $\mu_c$  from the raw couplings with the unstable FP-branch. Unlike for the model, in HN5 this is not merely provided by the intersection  $\kappa_0(\mu_c) = \kappa_-(\mu_c)$ , since HN5 possesses *two* renormalizable couplings,  $A_1$  and  $A_2$ , that form an unstable FB-manifold. As this FP is unstable, we proceed with a “shooting” and bi-sectioning approach where we evolve repeatedly the RG-flow from the raw couplings at some value of  $\mu$  and either increase or decrease  $\mu$  with ever smaller increments, depending on whether the RG-flow has reached a stable strong- or weak-coupling FP. After several iterations of this procedure, the RG-flow will remain near the unstable FP for many recursions, indicating that we are close to  $\mu_c$ .

We recall that the RG-recursions for  $A_1$  and  $A_2$ :

$$\{B_1, B_2\} /. RG_{h0}$$

$$\left\{ \frac{2(1+\mu)A_1A_2}{1+2\mu A_1+A_1^2}, \frac{\mu^{2y}(1+\mu)(1+A_1)^2}{2(1+2\mu A_1+A_1^2)} \right\}$$

In the following, we have already iterated by hand the “shooting” and bi-sectioning procedure and found a good approximation for  $\mu_c = 0.165805 \dots$  at  $y=0.1$ , confirmed by the fact that the RG-flow remains near the unstable FP for many recursions (only  $i=10$  are shown):

```
In[45]:= y = .1
μ = 0.165805160187
A1 = μ2
A2 = μ(2 y)
For[i = 0, i < 10, i++, Print[i, "    ", {A1, A2} = {B1, B2} /. RGh0]]
```

```
Out[45]= 0.1
```

```
Out[46]= 0.165805
```

```
Out[47]= 0.0274914
```

```
Out[48]= 0.698103
```

```
0    {0.0443104, 0.425408}
1    {0.0432307, 0.436516}
2    {0.0432979, 0.435808}
3    {0.0432937, 0.435852}
4    {0.043294, 0.435849}
5    {0.043294, 0.435849}
6    {0.043294, 0.435849}
7    {0.043294, 0.435849}
8    {0.043294, 0.435849}
9    {0.043294, 0.435849}
```

This value of  $\mu_c = 0.165805 \dots$  corresponds to a critical temperature of

```
In[50]:= Tc = -2 / Log[μ]
```

```
Out[50]= 1.113
```

In particular, at this  $\mu_c$ , we find the temperature exponent  $y_t = \log_2[\lambda_- (\mu_c)]$ :

```
In[51]:= yt = Log[EVh0[[1]]] / Log[2]
```

```
Out[51]= 0.0629237
```

and the magnetic exponent  $y_h = \log_2[\lambda_h (\mu_c)]$ :

```
In[52]:= yh = Log[(EVh→0)[[3]]] / Log[2]
```

```
Out[52]= 0.987091
```

From the scaling relation in Eq. (14) we finally obtain:

```
In[53]:= β = (1 - yh) / yt
```

```
Out[53]= 0.205158
```
