# Supplementary material for: Classification of critical phenomena in hierarchical small-world networks
Source: arXiv:1209.3447 source file (2015-05-08)
Supplement: Supplementary file 2 [file Landau_supplement.pdf]

# Supplement A:

## “Classification of Critical Phenomena having a Parameter-Dependent Renormalization ”

S. Boettcher and C. T. Brunson

---

### Eigenvalues of the Model in Eq. (5):

Eq. (5) provides our model:

$$\text{In}[1]:= \kappa_{n+1} = (1 - \kappa_B^2 + A^2 (\mu - \mu_B)) \kappa_n + 2 \kappa_B \kappa_n^2 - \kappa_n^3$$

$$\text{Out}[1]= (1 + A^2 (-\mu_B + \mu) - \kappa_B^2) \kappa_n + 2 \kappa_B \kappa_n^2 - \kappa_n^3$$

Note the explicit  $\mu$ -dependence in the equation.

We set  $\kappa_{n+1} = \kappa_n = \kappa_\infty$

$$\text{In}[2]:= \text{eqFP} = 0 == \text{Expand}[-\kappa_\infty + (\kappa_{n+1} /. \kappa_n \rightarrow \kappa_\infty)]$$

$$\text{Out}[2]= 0 == -\mu_B A^2 \kappa_\infty + A^2 \mu \kappa_\infty - \kappa_B^2 \kappa_\infty + 2 \kappa_B \kappa_\infty^2 - \kappa_\infty^3$$

to determine the fixed points of our theory,

$$\text{In}[3]:= \text{FP} = \text{Simplify}[\text{Solve}[\text{eqFP}, \kappa_\infty], \text{Assumptions} \rightarrow A > 0]$$

$$\text{Out}[3]= \left\{ \left\{ \kappa_\infty \rightarrow 0 \right\}, \left\{ \kappa_\infty \rightarrow -A \sqrt{-\mu_B + \mu} + \kappa_B \right\}, \left\{ \kappa_\infty \rightarrow A \sqrt{-\mu_B + \mu} + \kappa_B \right\} \right\}$$

To obtain each eigenvalue  $\lambda_0$ ,  $\lambda_-$ , and  $\lambda_+$ , we have to expand around the respective branch of  $\kappa_\infty$  in FP with  $\kappa_n \sim \kappa_\infty + \epsilon_n$  for  $\epsilon_n \ll 1$  to linearize the equation

$$\begin{aligned} \text{In}[4]:= & \epsilon_{n+1} = \text{Series}[-\kappa_\infty + \kappa_{n+1} /. \kappa_n \rightarrow (\kappa_\infty + \epsilon_n), \{\epsilon_n, 0, 1\}] \\ & \lambda_0 = \text{Collect}[\text{Coefficient}[\epsilon_{n+1} /. \text{FP}[[1]], \epsilon_n, 1], A] \\ & \lambda_- = \text{Collect}[\text{Coefficient}[\epsilon_{n+1} /. \text{FP}[[2]], \epsilon_n, 1], A, \text{Factor}] \\ & \lambda_+ = \text{Collect}[\text{Coefficient}[\epsilon_{n+1} /. \text{FP}[[3]], \epsilon_n, 1], A, \text{Factor}] \end{aligned}$$

$$\text{Out}[4]= (-\mu_B A^2 \kappa_\infty + A^2 \mu \kappa_\infty - \kappa_B^2 \kappa_\infty + 2 \kappa_B \kappa_\infty^2 - \kappa_\infty^3) + (1 - \mu_B A^2 + A^2 \mu - \kappa_B^2 + 4 \kappa_B \kappa_\infty - 3 \kappa_\infty^2) \epsilon_n + O[\epsilon_n]^2$$

$$\text{Out}[5]= 1 + A^2 (-\mu_B + \mu) - \kappa_B^2$$

$$\text{Out}[6]= 1 + 2 A^2 (\mu_B - \mu) + 2 A \sqrt{-\mu_B + \mu} \kappa_B$$

$$\text{Out}[7]= 1 + 2 A^2 (\mu_B - \mu) - 2 A \sqrt{-\mu_B + \mu} \kappa_B$$

which are the eigenvalues given in Eq. (7).

To reproduce Fig. 2(a), we plot those eigenvalues:

```

In[8]:= Show[
  Plot[1, {μ, -0.11, .4}, PlotStyle → {Dashed}],
  Plot[{λ0, λ-, λ+} /. κB → 1/2 /. "μB" → 0 /. A → 1,
    {μ, -0.11, .4}, ColorFunction → Function[{x, y}, If[y < 1, Black, Red]],
    ColorFunctionScaling → False, PlotStyle → {Thick}],
  PlotRange → {{-0.1, .4}, {0, 1.3}}, AxesLabel → {"μ-μB", "λ"}]

```

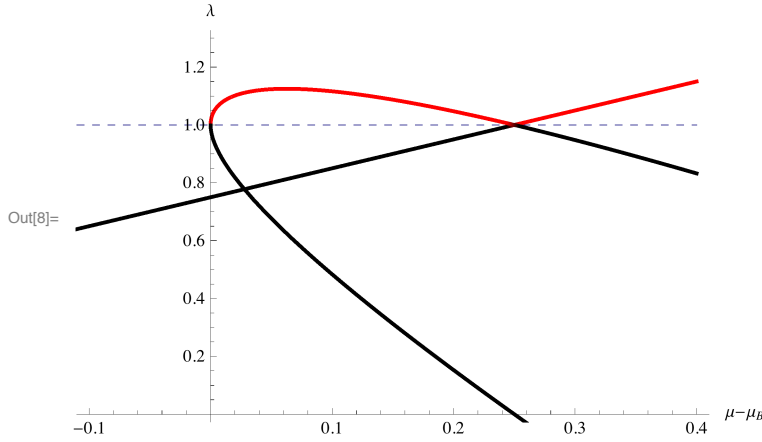

## Analysis of the case of Fig. 1(b):

```

In[9]:= Show[
  Plot[μ, {μ, 0, 1}, PlotStyle → {Green}],
  Plot[(κ∞ /. FP) /. κB → 1/3 /. "μB" → 1/9 /. A → 1/Sqrt[2], {μ, 0, 1}, ColorFunction →
    Function[{x, y}, If[(y < 1/3) && (y > 0) || ((y == 0) && (x > 1/3)), Red, Black]],
    ColorFunctionScaling → False, PlotStyle → {Thick}],
  PlotRange → {{0, 1}, {-0.03, 1}}, AxesLabel → {"μ", "κ"}]

```

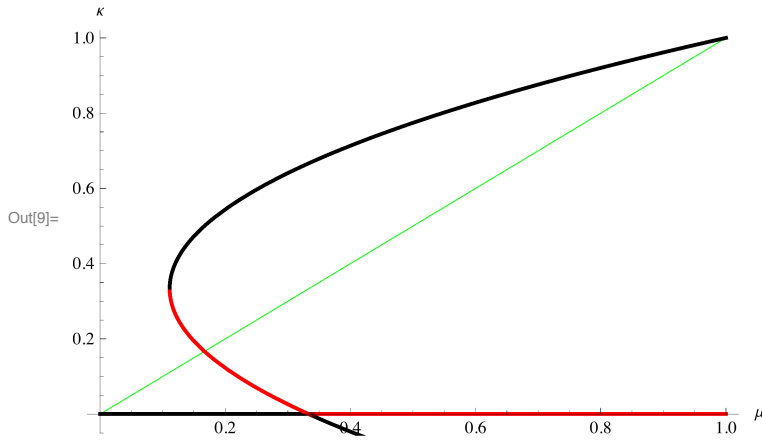

Here,  $\mu_c > \mu_B$  is located at the intersection of the (green) line  $\kappa_0 = \mu$  with  $\kappa_-(\mu)$ , i.e.,  $\kappa_-(\mu_c) = \mu_c$

```

In[10]:= μc = Solve[μ == (κ∞ /. FP)[[2]]], μ][[1]] /. μ → "μc"

```

$$\text{Out[10]} = \left\{ \mu_c \rightarrow \frac{1}{2} \left( A^2 + 2 \kappa_B - \sqrt{-4 \mu_B A^2 + A^4 + 4 A^2 \kappa_B} \right) \right\}$$

which is located at  $\mu_c = \frac{1}{6}$  in the example above:

```
In[11]:=  $\mu_c /. \kappa_B \rightarrow 1/3 /. "\mu_B" \rightarrow 1/9 /. A \rightarrow 1/\text{Sqrt}[2]$ 
```

```
Out[11]:=  $\left\{ \mu_c \rightarrow \frac{1}{6} \right\}$ 
```

We obtain the correlation length  $\xi$  in Eq. (8) with  $y_t = 1/\nu = \log_2 \lambda_-(\mu_c)$ , which for  $\mu_c \rightarrow \mu_B$  becomes

```
In[12]:=  $y_t = \text{Series}[\text{Log}[\lambda_-] / \text{Log}[2], \{\mu, "\mu_B", 1\}]$ 
```

```
Out[12]:=  $\frac{2 A \kappa_B \sqrt{\mu - \mu_B}}{\text{Log}[2]} - \frac{2 (A^2 + A^2 \kappa_B^2) (\mu - \mu_B)}{\text{Log}[2]} + O[\mu - \mu_B]^{3/2}$ 
```

hence,  $\nu \sim 1/\sqrt{\mu_c - \mu_B}$  for  $\mu_c \rightarrow \mu_B$ .

## Analysis of the case of Fig. 1(c):

```
In[13]:= Show[
  Plot[ $\mu$ , { $\mu$ , 0, 1}, PlotStyle -> {Green}],
  Plot[( $\kappa_\infty /. \text{FP}$ ) /.  $\kappa_B \rightarrow 1/4 /. "\mu_B" \rightarrow 1/2 /. A \rightarrow 3/\text{Sqrt}[8]$ , { $\mu$ , 0, 1}, ColorFunction ->
    Function[{x, y}, If[(y < 1/4) && (y > 0)] || ((y == 0) && (x > 0.56)), Red, Black]],
  ColorFunctionScaling -> False, PlotStyle -> {Thick}],
  PlotRange -> {{0, 1}, {-0.03, 1}}, AxesLabel -> {" $\mu$ ", " $\kappa$ "}
]
```

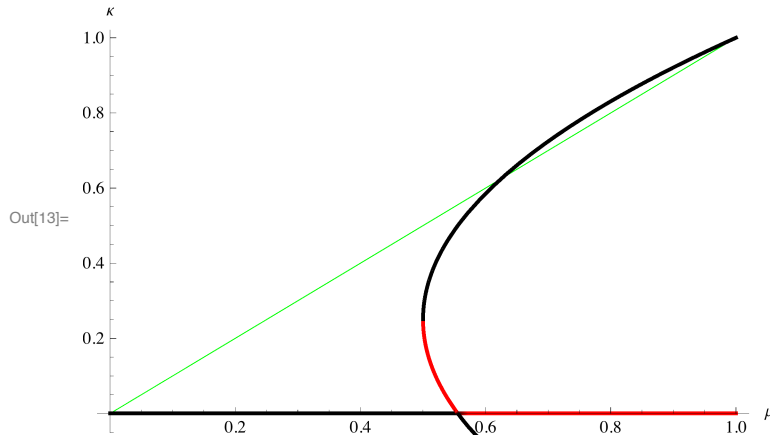

In this case, the critical point arises due to the RG-flow passing the branch point, i.e.,  $\mu_c = \mu_B (= \frac{1}{2})$  in the above plot). We obtain the correlation length  $\xi$  in Eq. (10) with the Ansatz near the branch point,  $\kappa_n \sim \kappa_B + \epsilon_n$  for  $\epsilon_n \ll 1$  simultaneously with  $\mu \rightarrow \mu_B + \Delta\mu$ , ( $\Delta\mu = \mu_B - \mu \ll 1$ ), expanded to 2nd order in  $\epsilon_n$  and 1st order in  $\Delta\mu$ :

```
In[14]:=  $\epsilon_{n+1} = \text{Simplify}[\text{Series}[-\kappa_B + \kappa_{n+1} /. \kappa_n \rightarrow (\kappa_B + \epsilon_n), \{\epsilon_n, 0, 2\}] /. \mu \rightarrow "\mu_B" - \Delta\mu]$ 
```

```
Out[14]:=  $-A^2 \Delta\mu \kappa_B + (1 - A^2 \Delta\mu) \epsilon_n - \kappa_B \epsilon_n^2 + O[\epsilon_n]^3$ 
```

The  $\Delta\mu$ -term in order- $\epsilon_n$  and any other higher-order term is irrelevant:

```
In[15]:=  $\epsilon_{n+1} = \text{Normal}[\epsilon_{n+1} + A^2 \Delta\mu \epsilon_n]$ 
```

```
Out[15]:=  $\epsilon_n - A^2 \Delta\mu \kappa_B - \epsilon_n^2 \kappa_B$ 
```

For large  $n$ , we approximate this non-linear recursion with a differential equation:

```
In[16]:= D[e[n], n] == Normal[εn+1 - εn] /. εn → e[n]
eqBKT = DSolve[%, e[n], n][[1]]
```

```
Out[16]:= e'[n] == -A2 Δμ κB - e[n]2 κB
```

```
Out[17]:= {e[n] → A √Δμ Tan[A √Δμ C[1] - A n √Δμ κB]}
```

For large  $n$ , the initial condition is clearly irrelevant:

```
In[18]:= eqBKT = eqBKT /. C[1] → 0
```

```
Out[18]:= {e[n] → -A √Δμ Tan[A n √Δμ κB]}
```

Thus, the solution for  $e[n] \sim \epsilon_n$  overruns its bound on a scale of  $n^* \sim 1 / \sqrt{\Delta\mu}$  for  $\Delta\mu \rightarrow 0$ , resulting in the BKT-divergence of the correlation-length in Eq. (10).

## Analysis of the case of Fig. 1(d):

```
In[19]:= Show[
  Plot[μ, {μ, 0, 1}, PlotStyle → {Green}],
  Plot[(κ∞ /. FP) /. κB → -1/8 /. "μB" → 1/2 /. A → Sqrt[2] * 9/8, {μ, 0, 1},
    ColorFunction → Function[{x, y}, If[(y == 0) && (x > 0.51)], Red, Black]],
    ColorFunctionScaling → False, PlotStyle → {Thick}],
  PlotRange → {{0, 1}, {-0.05, 1}}, AxesLabel → {"μ", "κ"}
]
```

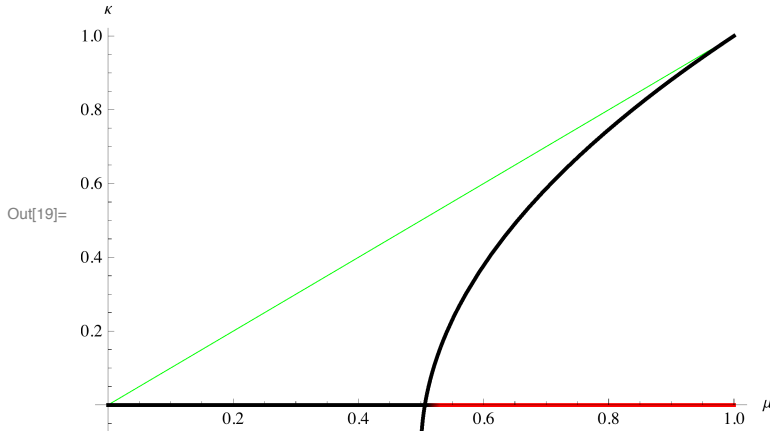

In this case,  $\kappa_B < 0$  and the critical point is located at the intersection of  $\kappa_\infty = 0$  and the upper branch of  $\kappa_\infty$ :

```
In[20]:= μc = Expand[Solve[(κ∞ /. FP[[1]]) == (κ∞ /. FP[[3]]), μ][[1]] /. μ → "μc"]
```

```
Out[20]:= {μc → μB + κB2 / A2}
```

which in the example in the plot above yields  $\mu_c \rightarrow \frac{41}{81}$ :

```
In[21]:= μc /. κB → -1/8 /. "μB" → 1/2 /. A → Sqrt[2] * 9/8
```

```
Out[21]:= {μc → 41/81}
```

We can determine the eigenvalues near  $\mu_c$  for the FP  $\kappa_\infty = 0$  and  $\kappa_\infty = \kappa_-$  by expanding  $\lambda_0$  and  $\lambda_-$  from Eqs. (7) for  $\Delta\mu = (\mu - \mu_c) \rightarrow 0$ :

```
In[22]:= Simplify[Series[ $\lambda_0$  /.  $\mu \rightarrow (" \mu_c" /. \mu_c) + \Delta\mu$ ], { $\Delta\mu$ , 0, 1}], Assumptions  $\rightarrow A > 0 \ \&\& \ \kappa_B > 0$ ]
Simplify[Series[ $\lambda_-$  /.  $\mu \rightarrow (" \mu_c" /. \mu_c) + \Delta\mu$ ], { $\Delta\mu$ , 0, 1}], Assumptions  $\rightarrow A > 0 \ \&\& \ \kappa_B > 0$ ]
```

```
Out[22]=  $1 + A^2 \Delta\mu + O[\Delta\mu]^2$ 
```

```
Out[23]=  $1 - A^2 \Delta\mu + O[\Delta\mu]^2$ 
```

Note that the FP  $\kappa_\infty = 0$  destabilizes for  $\mu$  approaching  $\mu_c$  from below ( $\Delta\mu < 0$ ) while the FP  $\kappa_\infty = \kappa_-$  destabilizes for  $\mu$  approaching  $\mu_c$  from above ( $\Delta\mu > 0$ ). Thus, the controlling eigenvalue on both sides is  $\lambda \sim 1 - A^2 |\Delta\mu|$  and for the size-crossover:

```
In[24]:=  $n_* = \text{Series}[1 / \text{Log}[1 - A^2 \Delta\mu], \{\Delta\mu, 0, -1\}]$ 
```

```
Out[24]=  $-\frac{1}{A^2 \Delta\mu} + O[\Delta\mu]^0$ 
```

resulting in Eq. (11).
